# Supplementary material for: Communication-free Massively Distributed Graph Generation
Source: arXiv:1710.07565 source file (2019-03-18)
Supplement: Supplementary file 1 [file app-additional-results.tex]

\section{Additional experimental results}
\begin{table}[h!]
	\begin{center}
		\input{results/table_compare.tex}
	\end{center}
	
	\vspace{2em}
	
	\caption{Comparison of generators for $n=2^{26}$, $\alpha \in \{0.55, 1\}$, and $\bar d \in \{10, 1000\}$.
		\textsl{Comp} refers to the number of distance computations between two points.
		It does not include node pairs that could be ruled out earlier (e.g., by comparing indices or radii).
		For \hypgen{} the value is higher due to vectorisation which often prevents such early discarding.
		\textsl{RSS} is the maximal resident set size (i.e. peak memory allocation) as reported by the operating system.
		In case of \rhg{} it is the sum of RSS of all MPI processes yielding a higher overhead.
		\girggen{} is a purely sequential implementation and includes fewer data points due to the high runtime.
		We report the standard deviation of the $S$ measurements as uncertainty and apply statistical error propagation.
		\\
		\vspace{0.5em}
		$\dagger$ Experiment was cancelled after a runtime of $10^5$~s.	
	}
	\label{tab:generator_compares}
\end{table}

\newcommand{\appScale}{0.63}

\begin{figure}
	\scalebox{\appScale}{\input{results/plot_gtime_d10_e21_abs.pgf}}
	\hfill
	\scalebox{\appScale}{\input{results/plot_gtime_d10_e21_rel.pgf}}

	\scalebox{\appScale}{\input{results/plot_gtime_d10_e30_abs.pgf}}
	\hfill
	\scalebox{\appScale}{\input{results/plot_gtime_d10_e30_rel.pgf}}

	\scalebox{\appScale}{\input{results/plot_gtime_d1000_e21_abs.pgf}}
	\hfill
	\scalebox{\appScale}{\input{results/plot_gtime_d1000_e21_rel.pgf}}

	\scalebox{\appScale}{\input{results/plot_gtime_d1000_e30_abs.pgf}}
	\hfill
	\scalebox{\appScale}{\input{results/plot_gtime_d1000_e30_rel.pgf}}
	
	\caption{Runtime of generators as function of the number $n$ of nodes.}
	\label{fig:runtimeofn}
\end{figure}

\begin{figure}
	\scalebox{\appScale}{\input{results/plot_ressize_d10_e21_abs.pgf}}
	\hfill
	\scalebox{\appScale}{\input{results/plot_ressize_d10_e21_rel.pgf}}
	
	\scalebox{\appScale}{\input{results/plot_ressize_d10_e30_abs.pgf}}
	\hfill
	\scalebox{\appScale}{\input{results/plot_ressize_d10_e30_rel.pgf}}
	
	\scalebox{\appScale}{\input{results/plot_ressize_d1000_e21_abs.pgf}}
	\hfill
	\scalebox{\appScale}{\input{results/plot_ressize_d1000_e21_rel.pgf}}
	
	\scalebox{\appScale}{\input{results/plot_ressize_d1000_e30_abs.pgf}}
	\hfill
	\scalebox{\appScale}{\input{results/plot_ressize_d1000_e30_rel.pgf}}
	
	\caption{Max. memory allocation of generators as function of the number $n$ of nodes.}
	\label{fig:ressizeofn}
\end{figure}
